# Supplementary material for: Pilot Clustering in Asymmetric Massive MIMO Networks
Source: arXiv:1507.03773 source file (2015-07-14)
Supplement: Supplementary file 1 [file appendix.tex]

\appendices

\section{Proof of Theorem \ref{theorem:sum-spectral-efficiency}}\label{sec:proofth1}

In the case of MRC, the expectations in \eqref{eq:SINR-value} can be computed directly, using the estimates in Lemma \ref{lemma:estimation}:
\begin{equation}
\begin{split}
\mathrm{SINR}_{jk} &= \frac{ \frac{ \rho^2 B M  }{ \sum_{\ell \in \Phi_j (\mathcal{C})}   \frac{\rho d_j(\vect{z}_{\ell k}) }{d_\ell(\vect{z}_{\ell k})} B + \sigma^2 } }{ \fracSum{l \in \Phi_j (\mathcal{C}) \setminus \{ j \}} 
   \frac{ \left( \frac{\rho d_j(\vect{z}_{lk}) }{ d_l(\vect{z}_{lk})} \right)^2 B M  }{ \sum_{\ell \in \Phi_j (\mathcal{C})}   \frac{\rho d_j(\vect{z}_{\ell k}) }{d_\ell(\vect{z}_{\ell k})} B + \sigma^2 } +
\fracSum{l \in \mathcal{L}} \fracSumtwo{m=1}{K_l} \frac{\rho d_j(\vect{z}_{lm}) }{ d_l(\vect{z}_{lm})} +  \sigma^2   } \\
  &= \frac{ 1 }{ \fracSum{l \in \Phi_j (\mathcal{C}) \setminus \{ j \}} 
 \left( \frac{ d_j(\vect{z}_{lk}) }{ d_l(\vect{z}_{lk})} \right)^2    + \left( \fracSum{\ell \in \Phi_j (\mathcal{C})}   \frac{ d_j(\vect{z}_{\ell k}) }{d_\ell(\vect{z}_{\ell k})}  + \frac{\sigma^2}{B \rho} \right) \left(
\fracSum{l \in \mathcal{L}} \fracSumtwo{m=1}{K_l} \frac{ d_j(\vect{z}_{lm}) }{M  d_l(\vect{z}_{lm})} +  \frac{\sigma^2}{M \rho} \right)  }
  \end{split}
\end{equation}
where the first equality follows from dividing all terms by $\mathbb{E}_{\{\vect{h}\}} \{ \| \vect{g}_{jk} \|^2\} $ and the second term follows from simple algebra. The expression in \eqref{eq:achievable-SINR-MR2} is obtained by considering an achievable lower bound $\mathbb{E}_{\{\vect{z}\}} \{\log_2(1+ \frac{1}{f(\{\vect{z}\})}) \} \geq \log_2(1+ \frac{1}{\mathbb{E}_{\{\vect{z}\}} \{ f(\{\vect{z}\}) \} }) $ where the expectation with respect to user positions are moved to the denominator of the SINRs. 
It only remains to identify terms of the type in \eqref{eq:mu-definition1}--\eqref{eq:mu-definition2}, check how many UEs that are active in each cell, and to reorganize the terms.

Similarly, the expectations in \eqref{eq:SINR-value} can be computed for ZFC as
\begin{equation}
\begin{split}
&\mathrm{SINR}_{jk}  \\&= \frac{ \frac{\rho}{d_j(\vect{z}_{jk})} }{ 
\fracSum{l \in \Phi_j (\mathcal{C}) \setminus \{ j \}}  \frac{\rho}{d_l(\vect{z}_{lk})}
 \frac{ (d_j(\vect{z}_{lk}) )^2}{ d_j(\vect{z}_{jk}) d_l(\vect{z}_{lk})}   +
 \left(
 \fracSum{l \in \mathcal{L} } \fracSumtwo{m=1}{K_l} \frac{\rho d_j(\vect{z}_{lm}) }{  d_l(\vect{z}_{lm})} 
-
  \fracSum{l \in \Phi_j (\mathcal{C})} \fracSumtwo{m=1}{K_l} \frac{ \left(\frac{\rho d_j(\vect{z}_{lm}) }{  d_l(\vect{z}_{lm})}  \right)^2  B   }{ \fracSum{\ell \in \Phi_j (\mathcal{C})}   \frac{\rho d_j(\vect{z}_{\ell m}) }{d_\ell(\vect{z}_{\ell m})} B + \sigma^2 }
 +  \sigma^2 \right) \left( \frac{ \fracSum{\ell \in \Phi_j (\mathcal{C})}   \frac{\rho d_j(\vect{z}_{\ell k}) }{d_\ell(\vect{z}_{\ell k})} B + \sigma^2 }{ \rho  d_j(\vect{z}_{jk}) B (M - K_j)  }  \right) } \\
 & = \frac{ 1 }{ 
\fracSum{l \in \Phi_j (\mathcal{C}) \setminus \{ j \}}   \left(
 \frac{ d_j(\vect{z}_{lk}) }{ d_l(\vect{z}_{lk})} \right)^2  +
 \left(
 \fracSum{l \in \mathcal{L} } \fracSumtwo{m=1}{K_l} \frac{ d_j(\vect{z}_{lm}) }{  d_l(\vect{z}_{lm})} 
- \fracSum{l \in \Phi_j (\mathcal{C})} \fracSumtwo{m=1}{K_l}
  \frac{  \left(\frac{ d_j(\vect{z}_{lm}) }{  d_l(\vect{z}_{lm})}  \right)^2     }{ \fracSum{\ell \in \Phi_j (\mathcal{C})}   \frac{ d_j(\vect{z}_{\ell m}) }{d_\ell(\vect{z}_{\ell m})} + \frac{\sigma^2}{B \rho} }
 +  \frac{\sigma^2}{\rho} \right) \left( \frac{ \fracSum{\ell \in \Phi_j (\mathcal{C})}   \frac{ d_j(\vect{z}_{\ell k}) }{d_\ell(\vect{z}_{\ell k})} + \frac{\sigma^2}{B \rho} }{   M - K_j  }  \right) }
  \end{split}
\end{equation}
by using the zero-forcing definition and by utilizing well-known properties of Wishart matrices (see e.g.,
\cite[Proof of Proposition 2]{Ngo2013a}). Next, we use Jensen's inequality in the same way as for MRC to move the expectation with respect to user positions to the denominator of the SINRs.
Finally, \eqref{eq:achievable-SINR-ZF2} follows from identifying the propagation parameters \eqref{eq:mu-definition1}--\eqref{eq:mu-definition2}, and using the bound
\begin{equation}
\mathbb{E}_{\{\vect{z}\}} \left\{ - \left(\frac{ d_j(\vect{z}_{lm}) }{  d_l(\vect{z}_{lm})}  \right)^2
 \frac{  \fracSum{\ell \in \Phi_j (\mathcal{C})}   \frac{ d_j(\vect{z}_{\ell k}) }{d_\ell(\vect{z}_{\ell k})} + \frac{\sigma^2}{B \rho}    }{ \fracSum{\ell \in \Phi_j (\mathcal{C})}   \frac{ d_j(\vect{z}_{\ell m}) }{d_\ell(\vect{z}_{\ell m})} + \frac{\sigma^2}{B \rho} }
 \right\} \leq - (\mu_{jl}^{(1)})^2
\frac{  \fracSum{\ell \in \Phi_j (\mathcal{C})} \mu_{j \ell}^{(1)}  + \frac{\sigma^2}{ B \rho}  }{   \fracSum{\ell \in \Phi_j (\mathcal{C})} \mu_{j \ell}^{(1)}  + \frac{\sigma^2}{ B \rho} },
\end{equation}
where the inequality is once again from Jensen's inequality.
